# Supplementary material for: DenoiSeg: Joint Denoising and Segmentation
Source: arXiv:2005.02987 source file (2020-06-10)
Supplement: Supplementary file 1 [file supplement.tex]

\documentclass[runningheads]{llncs}
\usepackage{amsmath,graphicx}
\usepackage{textcomp} 
\usepackage{xspace} 
\usepackage{tikz}
\usepackage{xcolor}
\usepackage{marvosym}
\usepackage{tabularx}\usepackage{fancyhdr}

\makeatletter
\DeclareRobustCommand\onedot{\futurelet\@let@token\@onedot}
\def\@onedot{\ifx\@let@token.\else.\null\fi\xspace}

\newcommand{\DenoiSeg}{\mbox{\textsc{DenoiSeg}}\xspace}

% tabular
\usepackage{array}
\newcolumntype{L}[1]{>{\raggedright\let\newline\\\arraybackslash\hspace{0pt}}m{#1}}
\newcolumntype{C}[1]{>{\centering\let\newline\\\arraybackslash\hspace{0pt}}m{#1}}
\newcolumntype{R}[1]{>{\raggedleft\let\newline\\\arraybackslash\hspace{0pt}}m{#1}}

\pagestyle{fancy}
\fancyhf{}
\rhead{}
\lhead{Supplementary -- \DenoiSeg: Joint Denoising and Segmentation}
\rfoot{\thepage}

% ======================================================================================
% ======================================== 1 ===========================================
% ====================================================================================== 
\newcommand\figFlyWing{
\begin{figure}[!h]
    \centering
    \begin{minipage}{.03\linewidth}
    \begin{tikzpicture}
            \draw (0, 0) node[rotate=90] {\textcolor{white}{w}Fly Wing n20};
        \end{tikzpicture}
    \end{minipage}
    \begin{minipage}{.96\linewidth}
        \includegraphics[width=.49\linewidth,trim={0.6cm 1.3cm 0.6cm 0.5cm},clip]{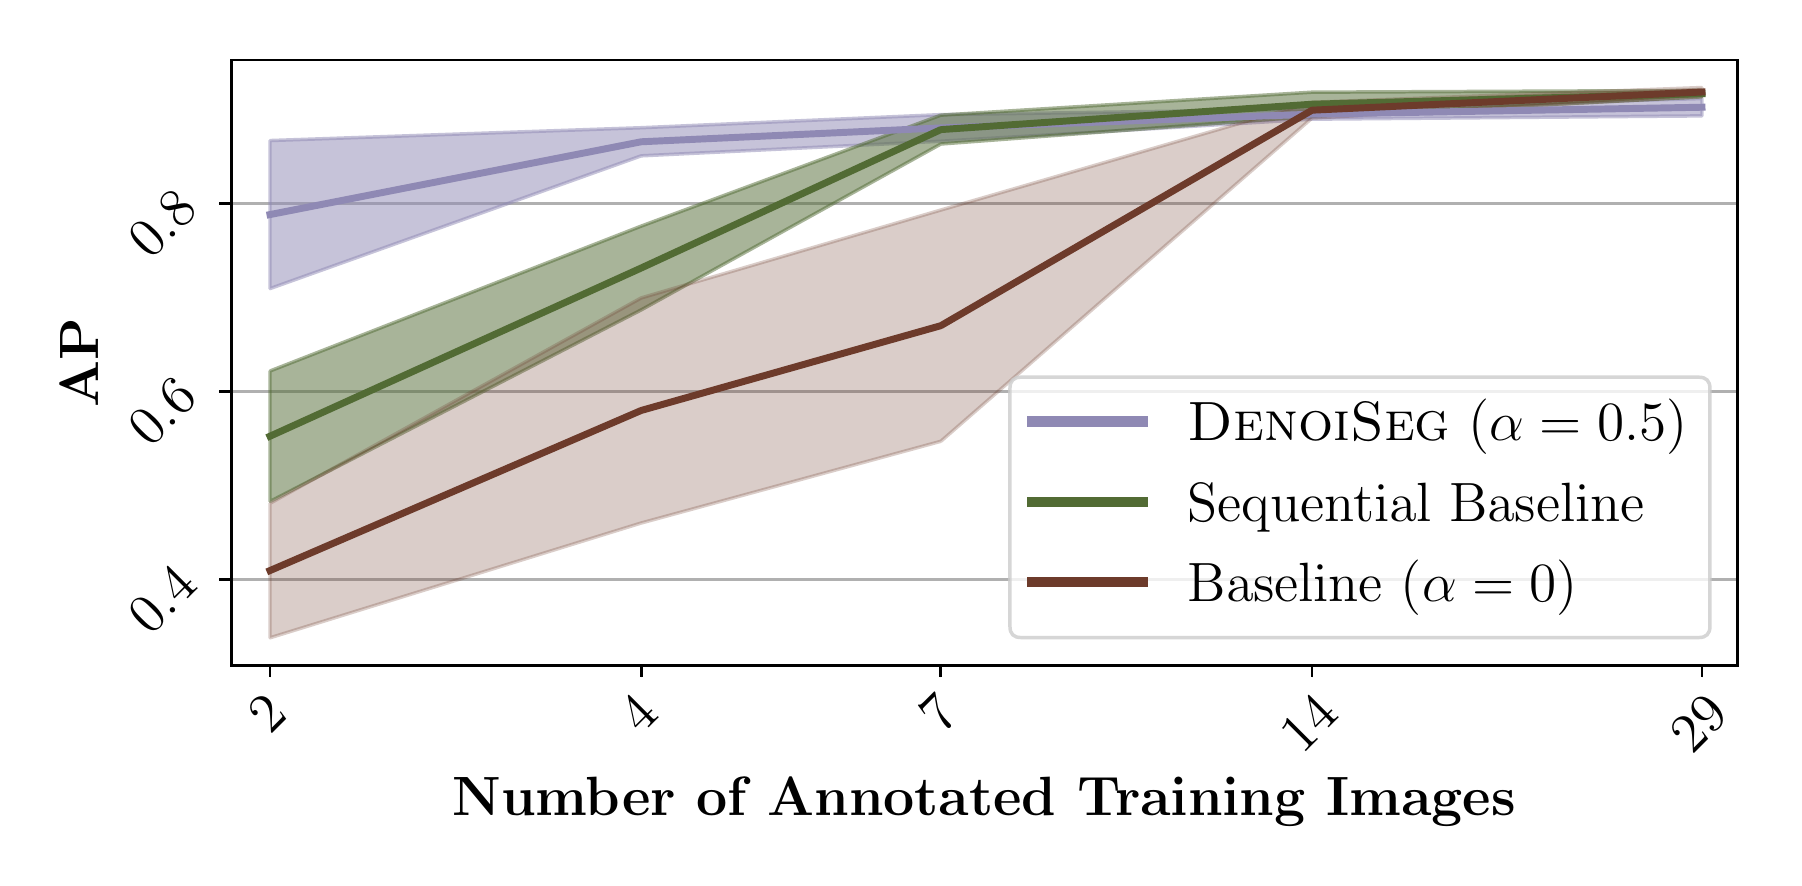}
        \includegraphics[width=.49\linewidth,trim={0.6cm 1.3cm 0.6cm 0.5cm},clip]{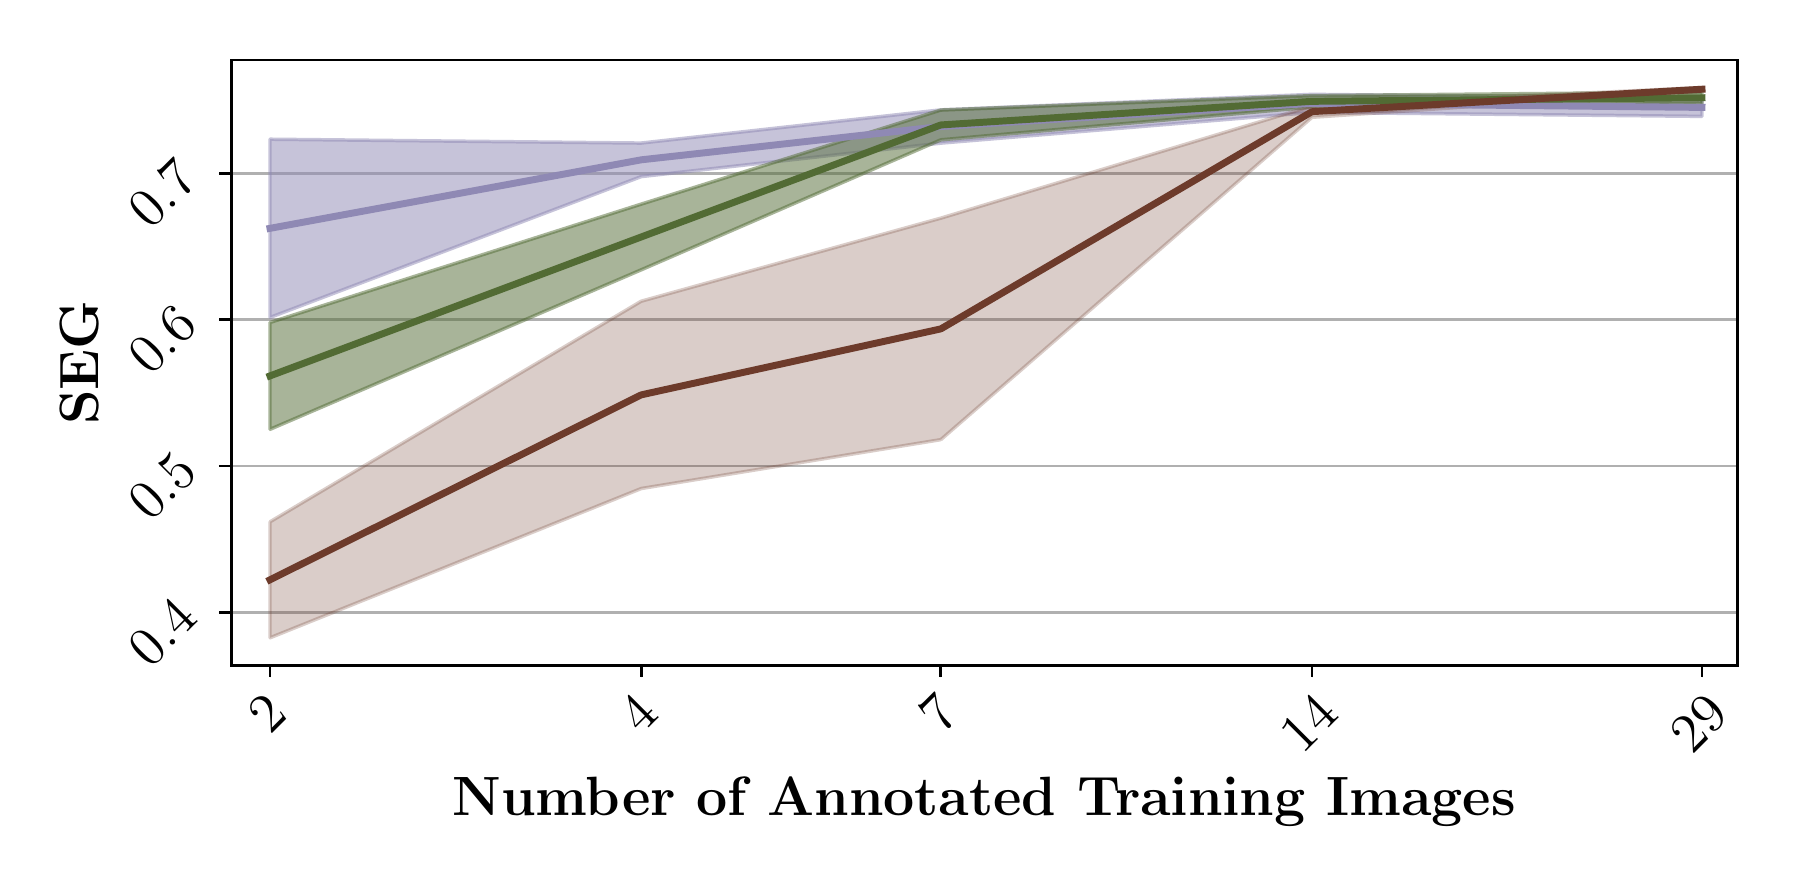}
    \end{minipage}

    \begin{minipage}{.03\linewidth}
    \begin{tikzpicture}
            \draw (0, 0) node[rotate=90] {\textcolor{white}{w}Fly Wing n10};
        \end{tikzpicture}
    \end{minipage}
    \begin{minipage}{.96\linewidth}
        \includegraphics[width=.49\linewidth,trim={0.6cm 1.3cm 0.6cm 0.5cm},clip]{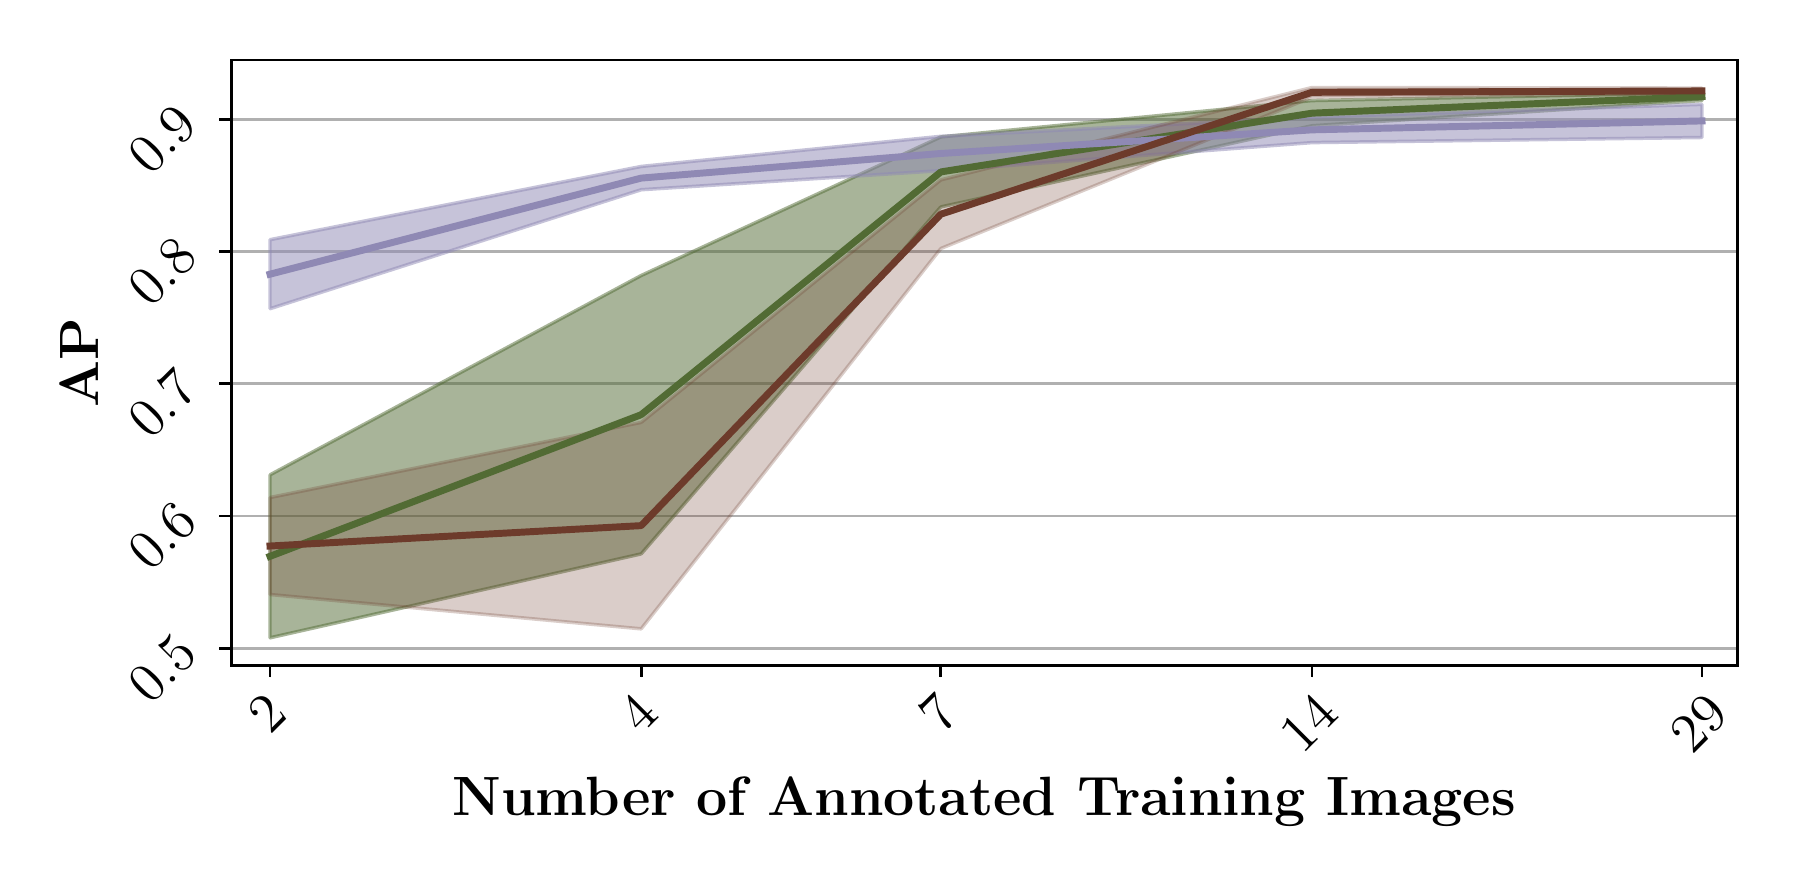}
        \includegraphics[width=.49\linewidth,trim={0.6cm 1.3cm 0.6cm 0.5cm},clip]{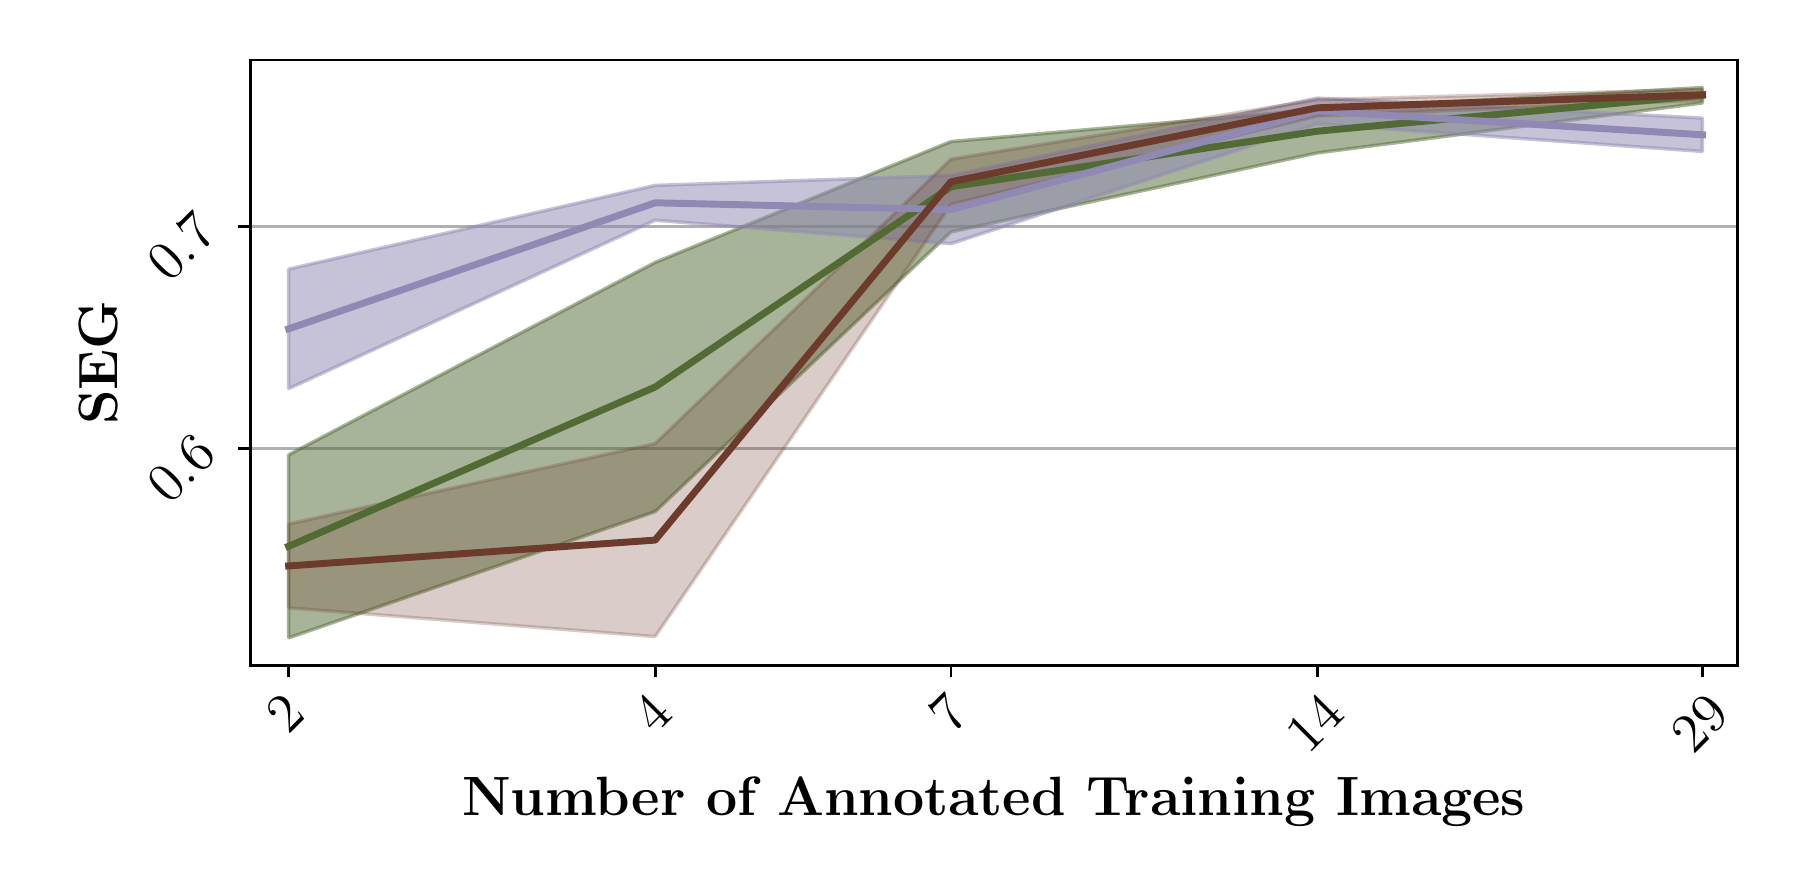}
    \end{minipage}

    \begin{minipage}{.03\linewidth}
    \begin{tikzpicture}
            \draw (0, 0) node[rotate=90] {\textcolor{white}{ws}Fly Wing n0}; % some whitespace to move the label up
        \end{tikzpicture}
    \end{minipage}
    \begin{minipage}{.96\linewidth}
        \includegraphics[width=.49\linewidth,trim={0.6cm 0.6cm 0.6cm 0.5cm},clip]{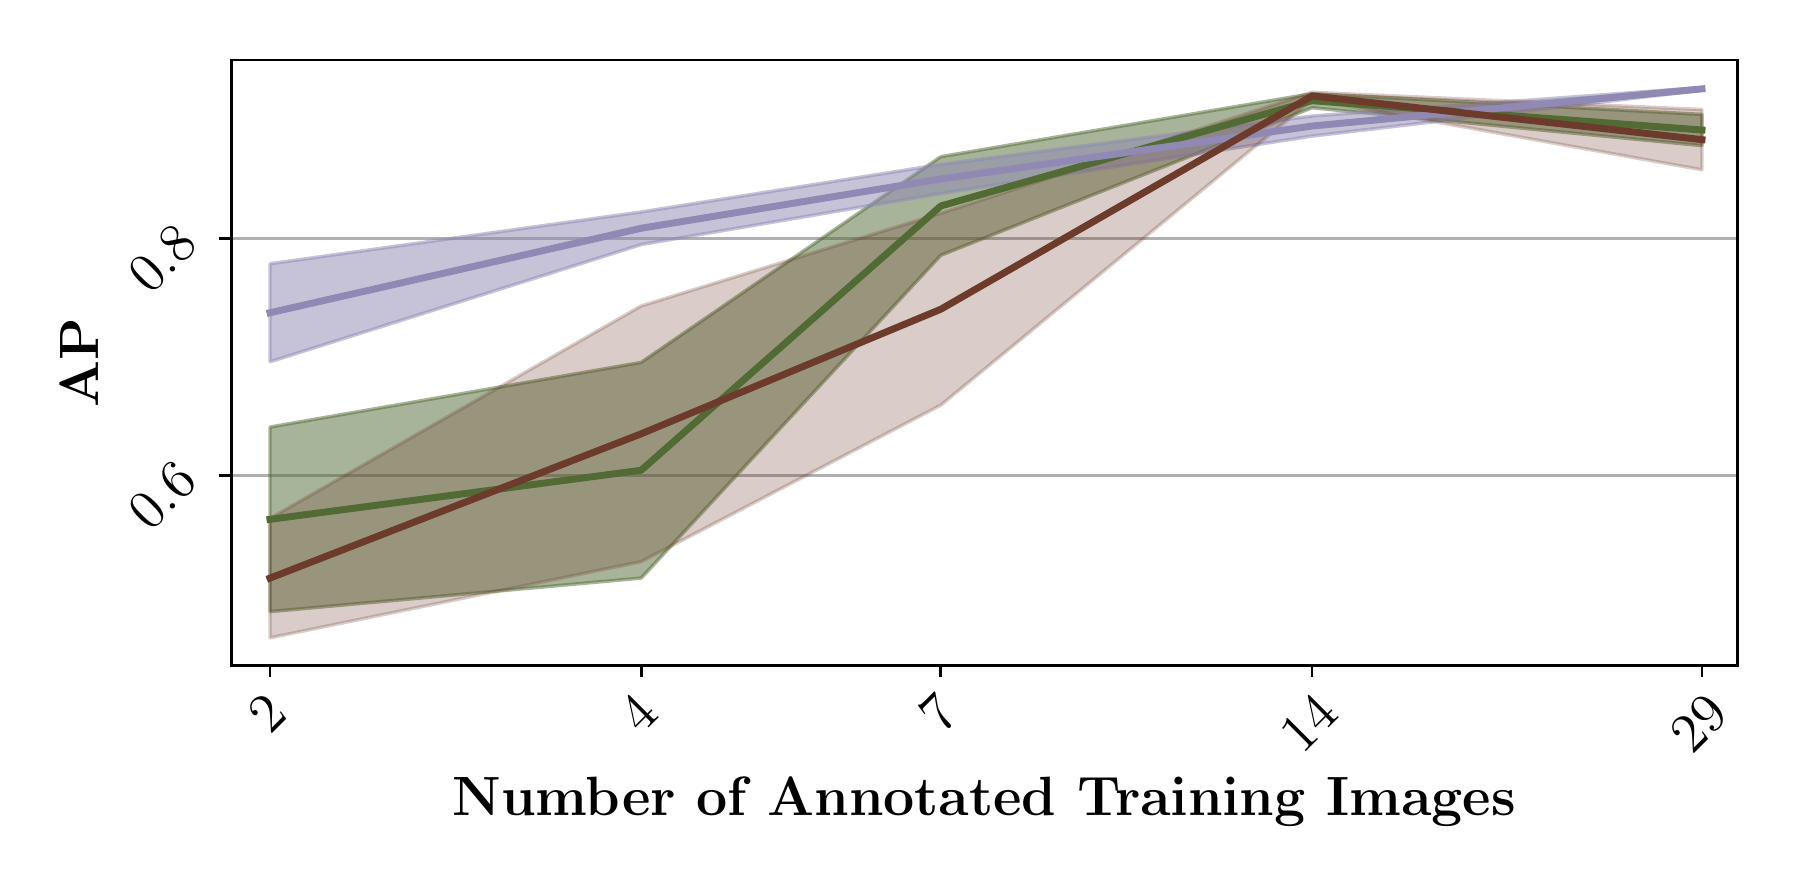}
        \includegraphics[width=.49\linewidth,trim={0.6cm 0.6cm 0.6cm 0.5cm},clip]{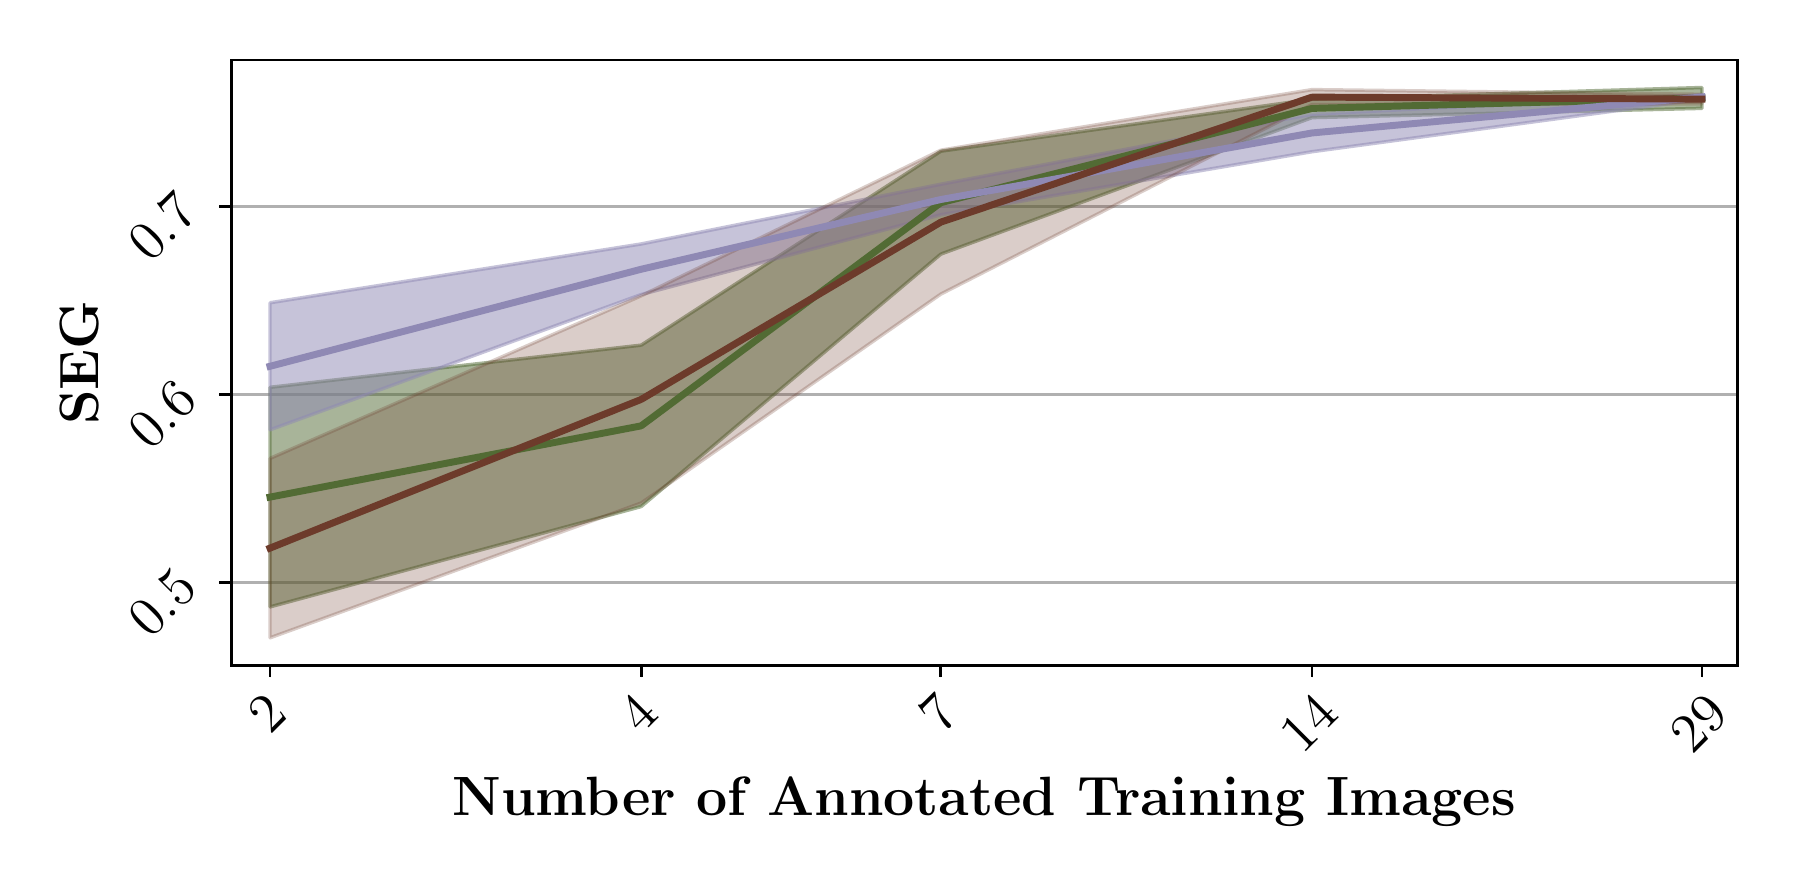}
    \end{minipage}
    
    \caption{Results for Fly Wing n0, n10, n20 data evaluated with AP and SEG-Score.}
    \label{fig:flywing}
\end{figure}
}

\newcommand\figMouseNuclei{
\begin{figure}[!h]
    \centering
    \begin{minipage}{.03\linewidth}
    \begin{tikzpicture}
            \draw (0, 0) node[rotate=90] {\textcolor{white}{w}Mouse n20};
        \end{tikzpicture}
    \end{minipage}
    \begin{minipage}{.96\linewidth}
        \includegraphics[width=.49\linewidth,trim={0.6cm 1.3cm 0.6cm 0.5cm},clip]{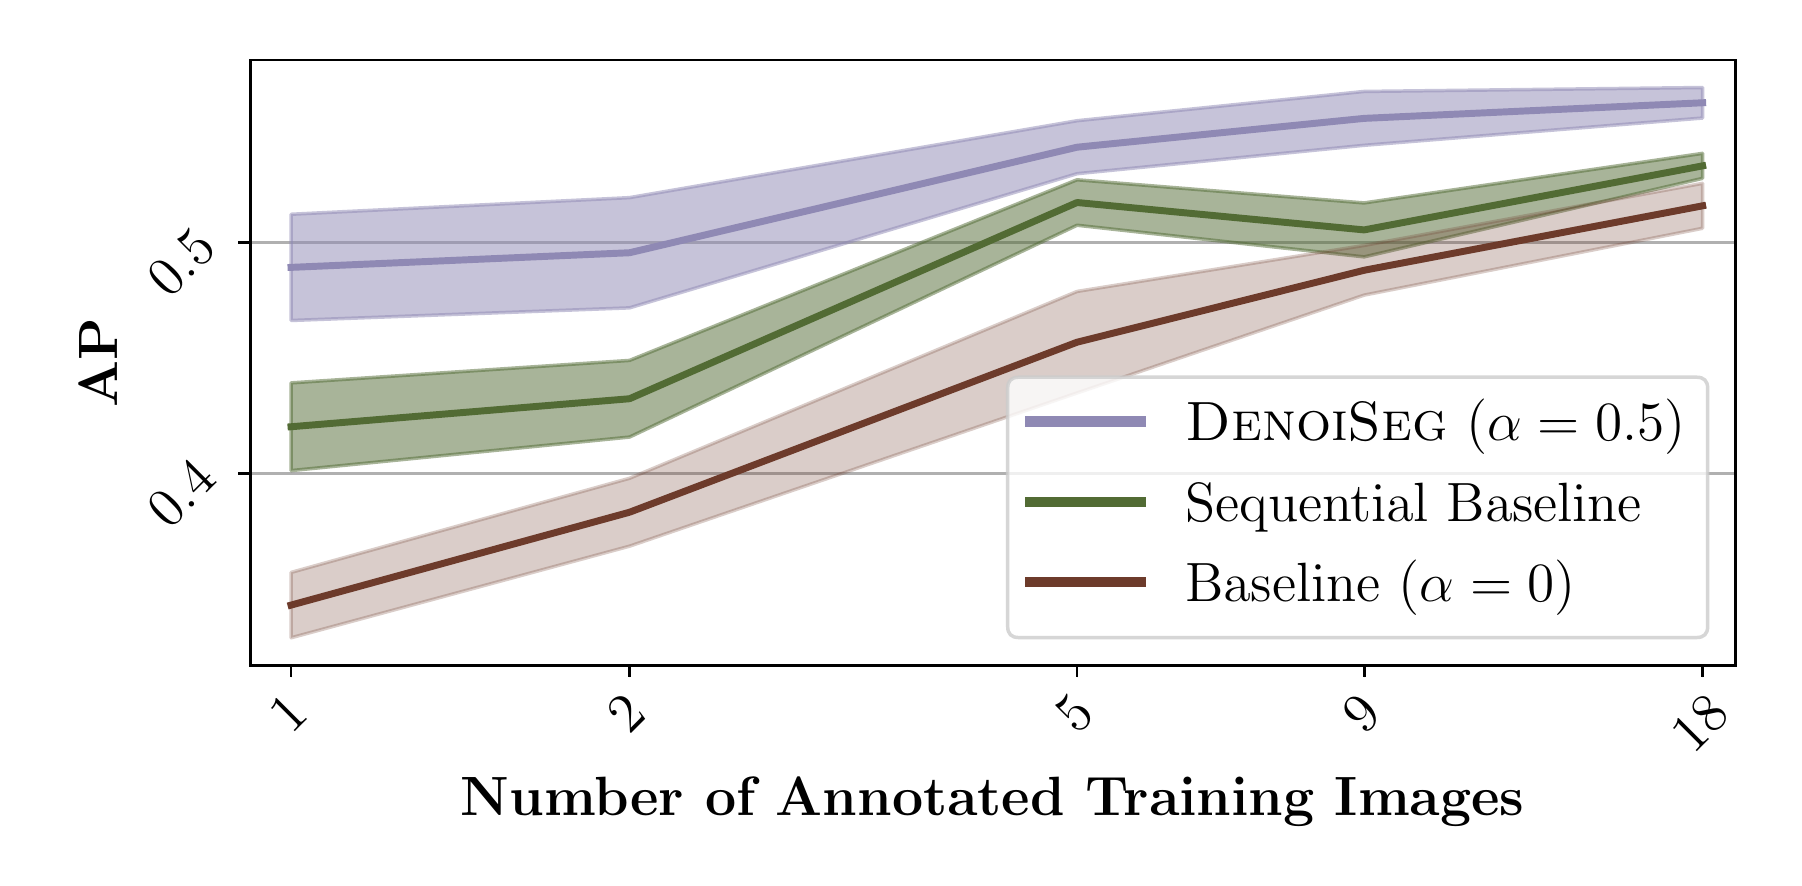}
        \includegraphics[width=.49\linewidth,trim={0.6cm 1.3cm 0.6cm 0.5cm},clip]{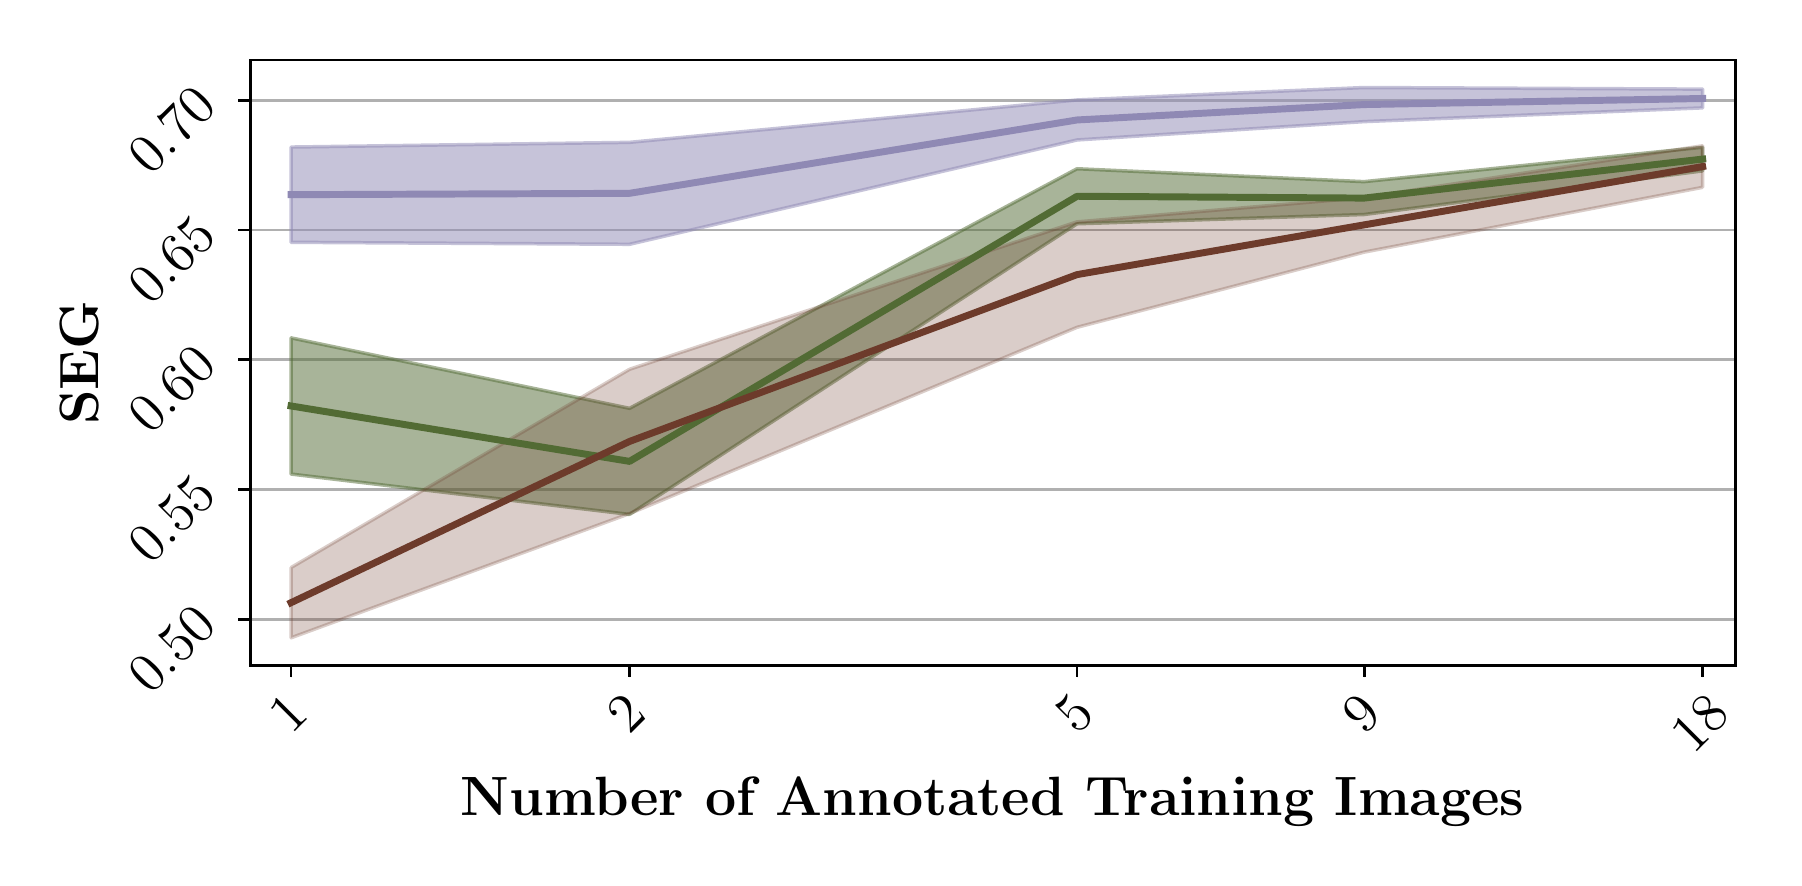}
    \end{minipage}

    \begin{minipage}{.03\linewidth}
    \begin{tikzpicture}
            \draw (0, 0) node[rotate=90] {\textcolor{white}{w}Mouse n10};
        \end{tikzpicture}
    \end{minipage}
    \begin{minipage}{.96\linewidth}
        \includegraphics[width=.49\linewidth,trim={0.6cm 1.3cm 0.6cm 0.5cm},clip]{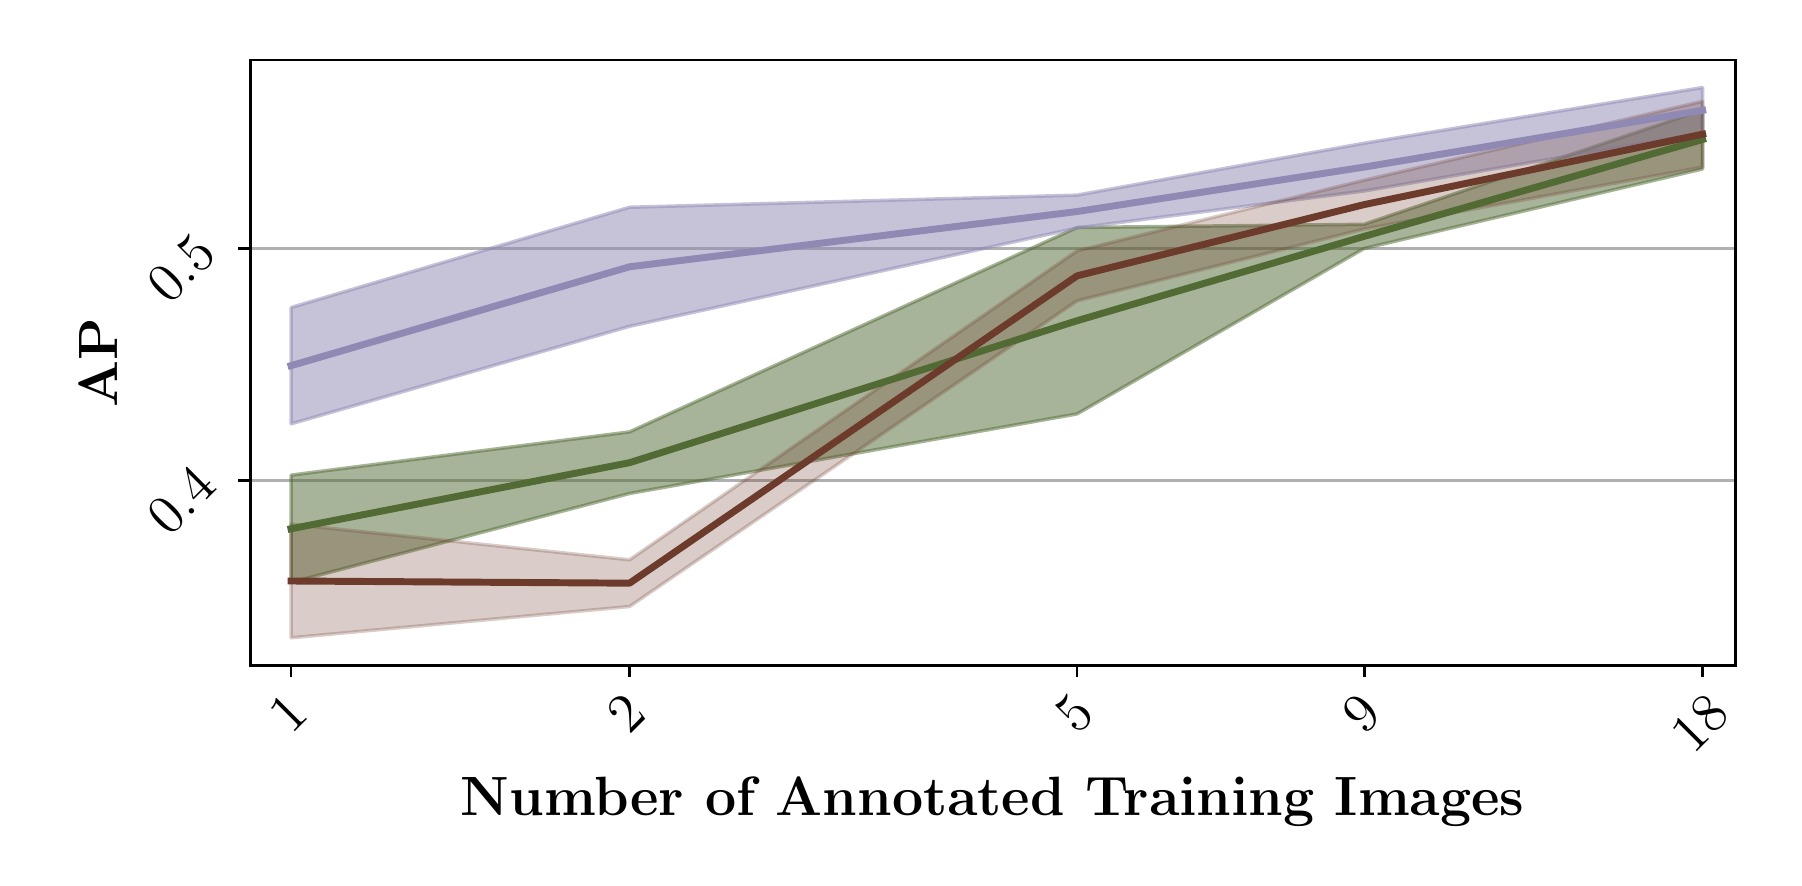}
        \includegraphics[width=.49\linewidth,trim={0.6cm 1.3cm 0.6cm 0.5cm},clip]{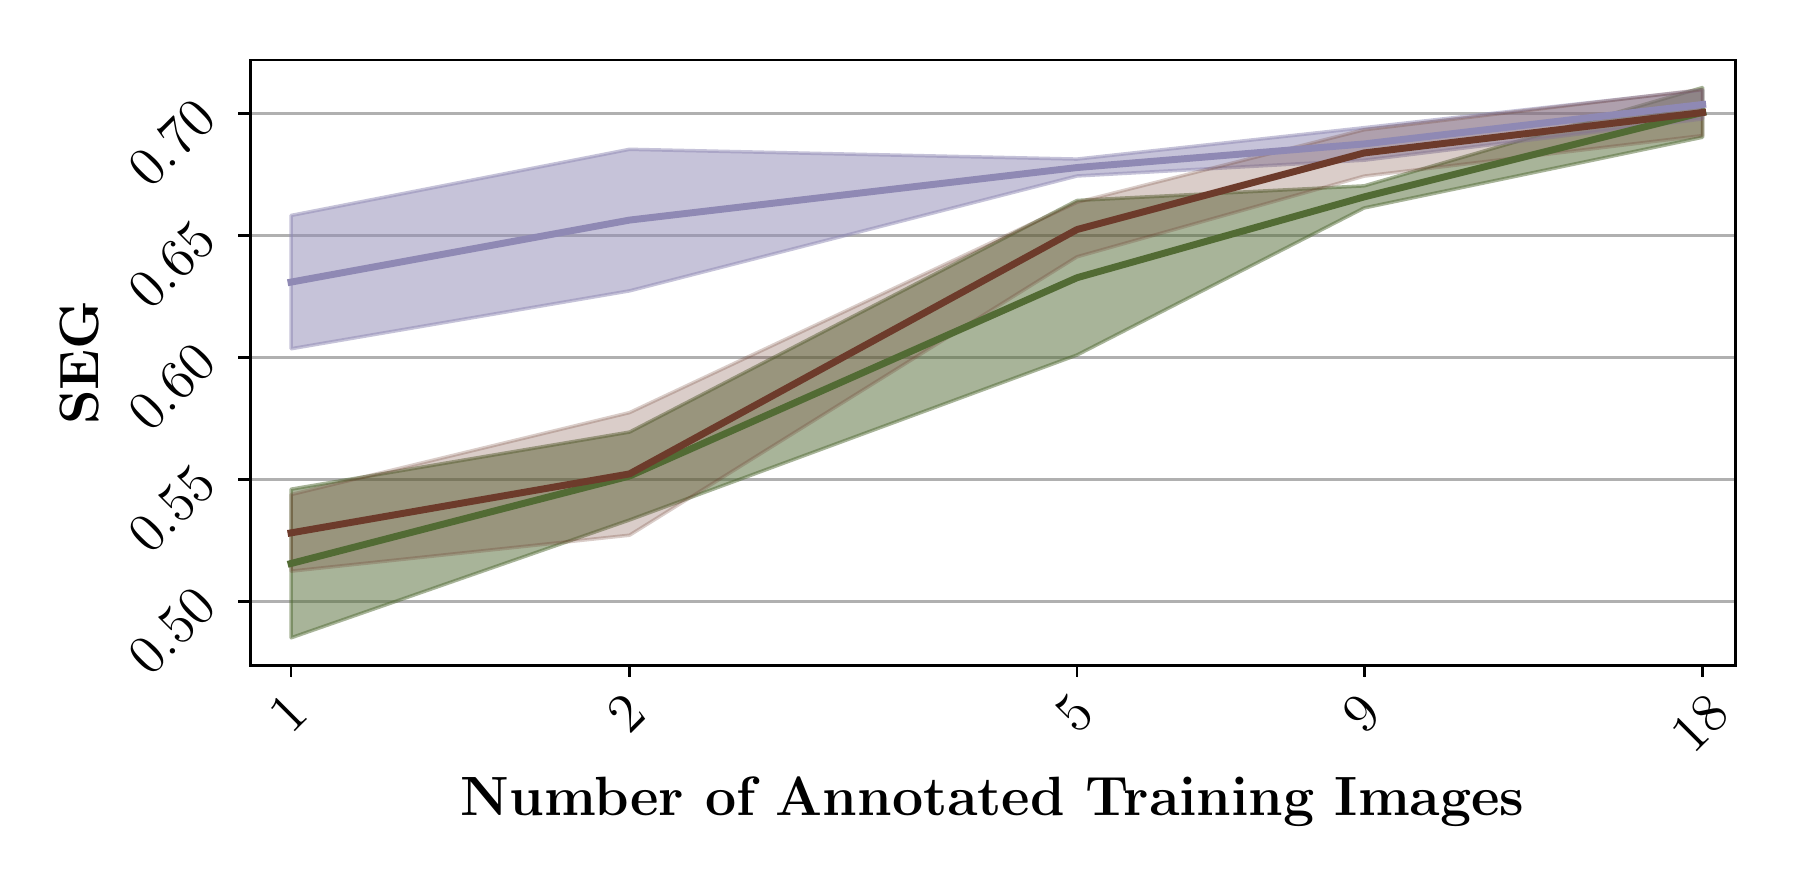}
    \end{minipage}

    \begin{minipage}{.03\linewidth}
    \begin{tikzpicture}
            \draw (0, 0) node[rotate=90] {\textcolor{white}{ws}Mouse n0}; % some whitespace to move the label up
        \end{tikzpicture}
    \end{minipage}
    \begin{minipage}{.96\linewidth}
        \includegraphics[width=.49\linewidth,trim={0.6cm 0.6cm 0.6cm 0.5cm},clip]{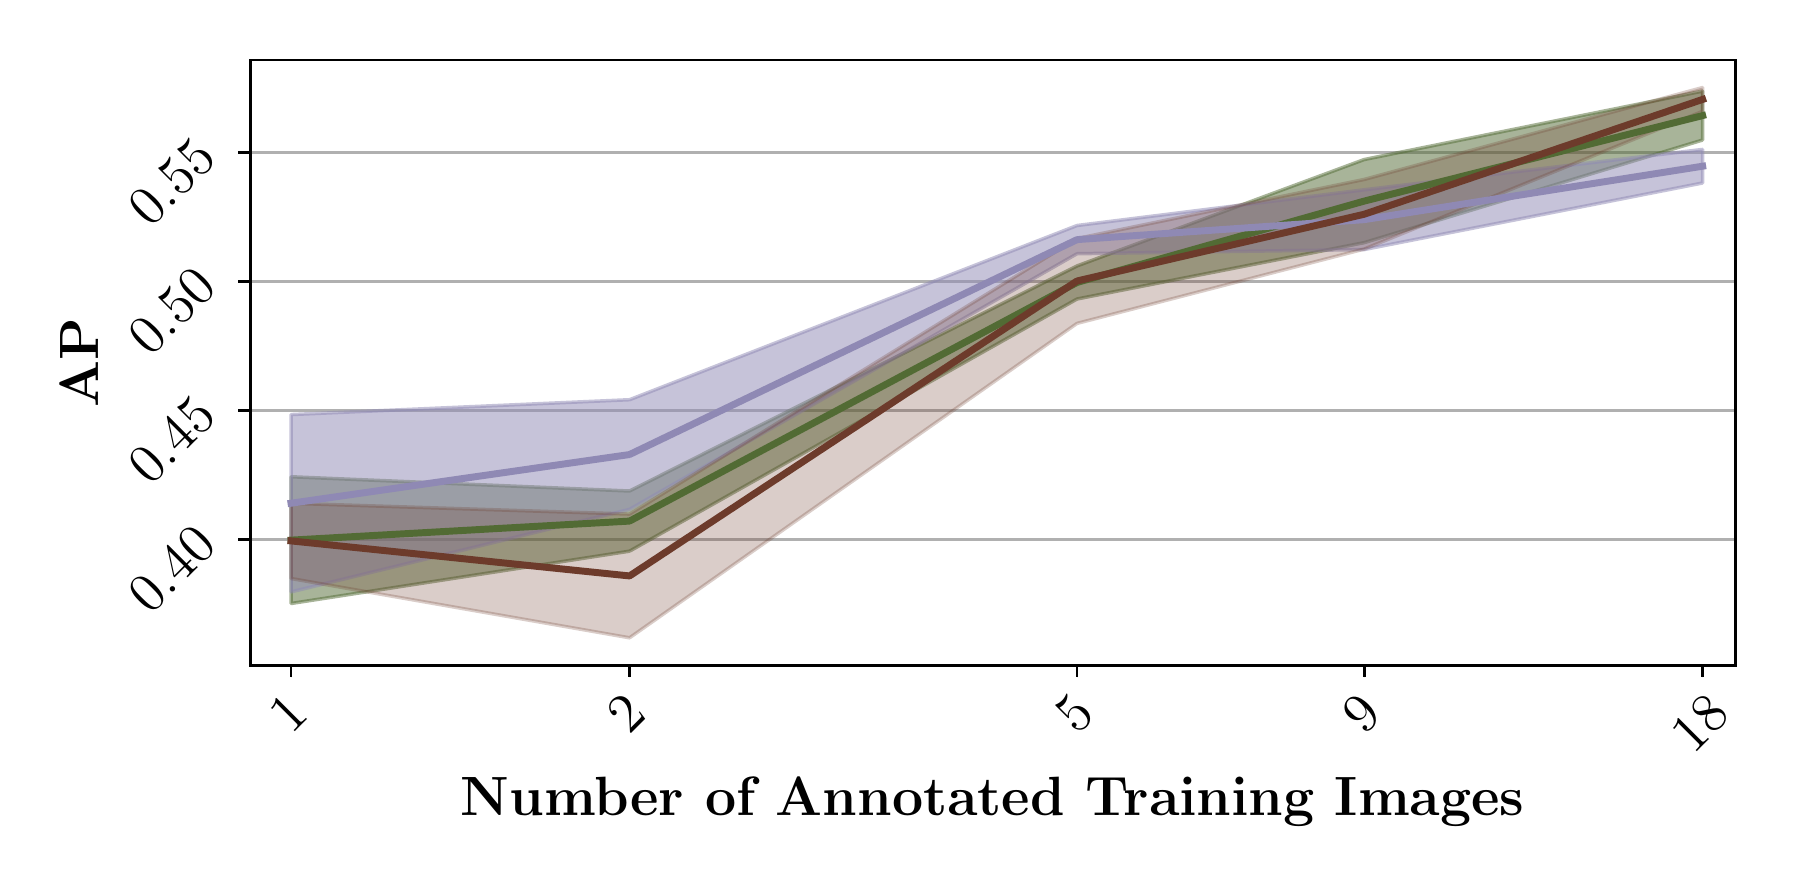}
        \includegraphics[width=.49\linewidth,trim={0.6cm 0.6cm 0.6cm 0.5cm},clip]{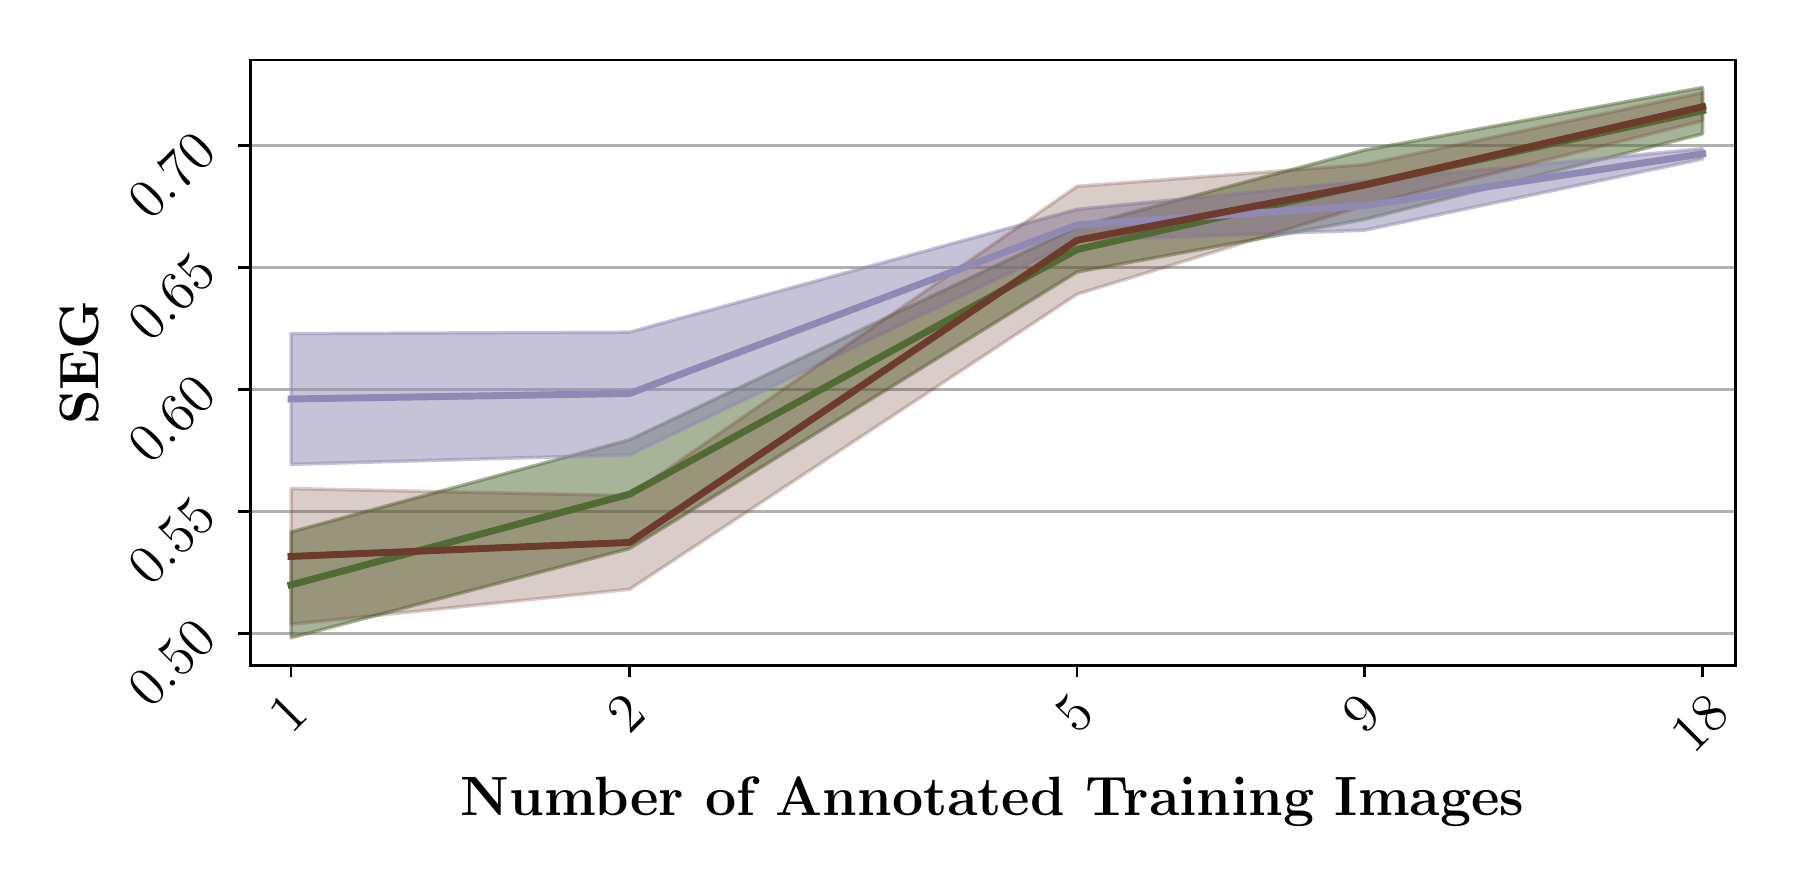}
    \end{minipage}
    
    \caption{Results for Mouse Nuclei n0, n10, n20 data evaluated with AP and SEG-Score.}
    \label{fig:mousenuclei}
\end{figure}
}

% ======================================================================================
% ======================================== 2 ===========================================
% ====================================================================================== 
\newcommand\figDelta{
\begin{figure}[!h]
    \centering
    \begin{minipage}{\linewidth}
        \begin{tikzpicture}
            \draw (0, 0) node[inner sep=0] {\includegraphics[width=.94\linewidth,trim={0.6cm 0.6cm 0.2cm 0.5cm},clip]{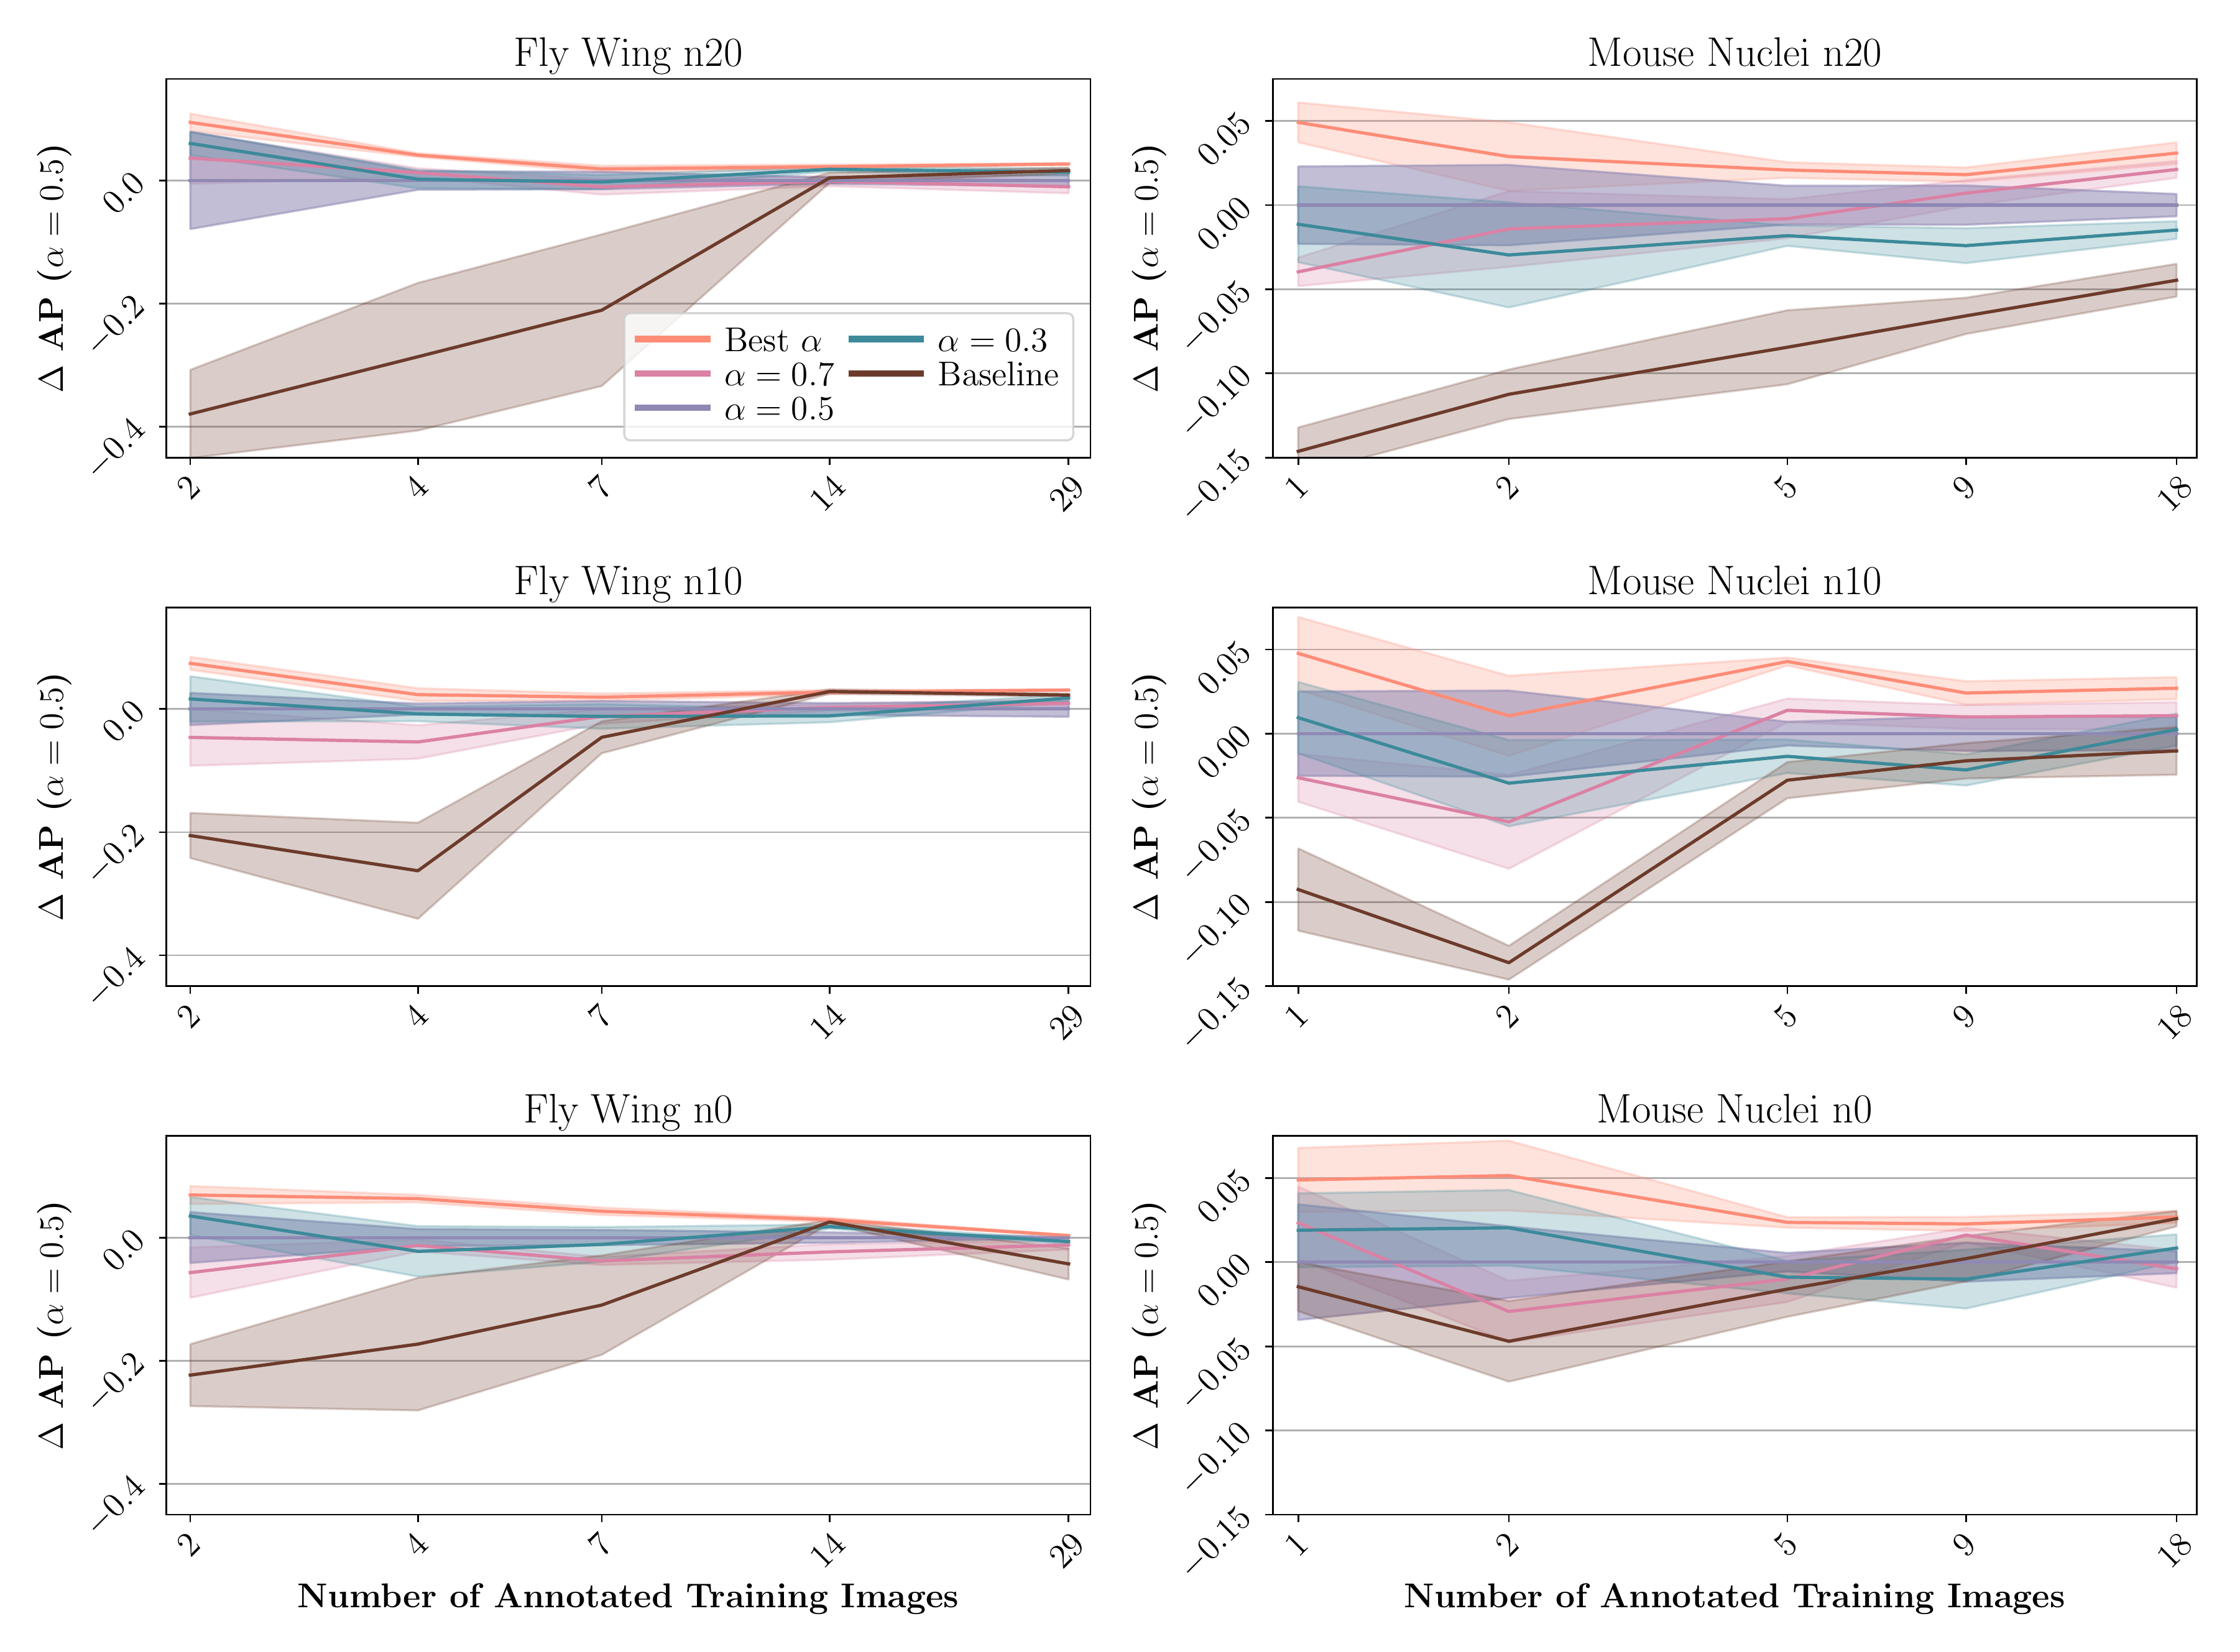}};
            \draw (-5.4, 4.2) node[inner sep=0] {(a)};
            \draw (0.35, 4.2) node[inner sep=0] {(b)};
        \end{tikzpicture}
    \end{minipage}
    
    \caption{Sensitivity of hyperparameter $\alpha$ for
    \textbf{(a)}~Fly Wing and \textbf{(b)}~Mouse Nuclei.}
    \label{fig:deltaNoise}
\end{figure}
}

% ======================================================================================
% ======================================== 3 ===========================================
% ====================================================================================== 
\newcommand\figVanillaBaseline{
\begin{figure}[!h]
    \centering
    \begin{minipage}{\linewidth}
        \begin{tikzpicture}
            \draw (0, 0) node[inner sep=0] {\includegraphics[width=.94\linewidth,trim={0.6cm 0.5cm 0.2cm 0.5cm},clip]{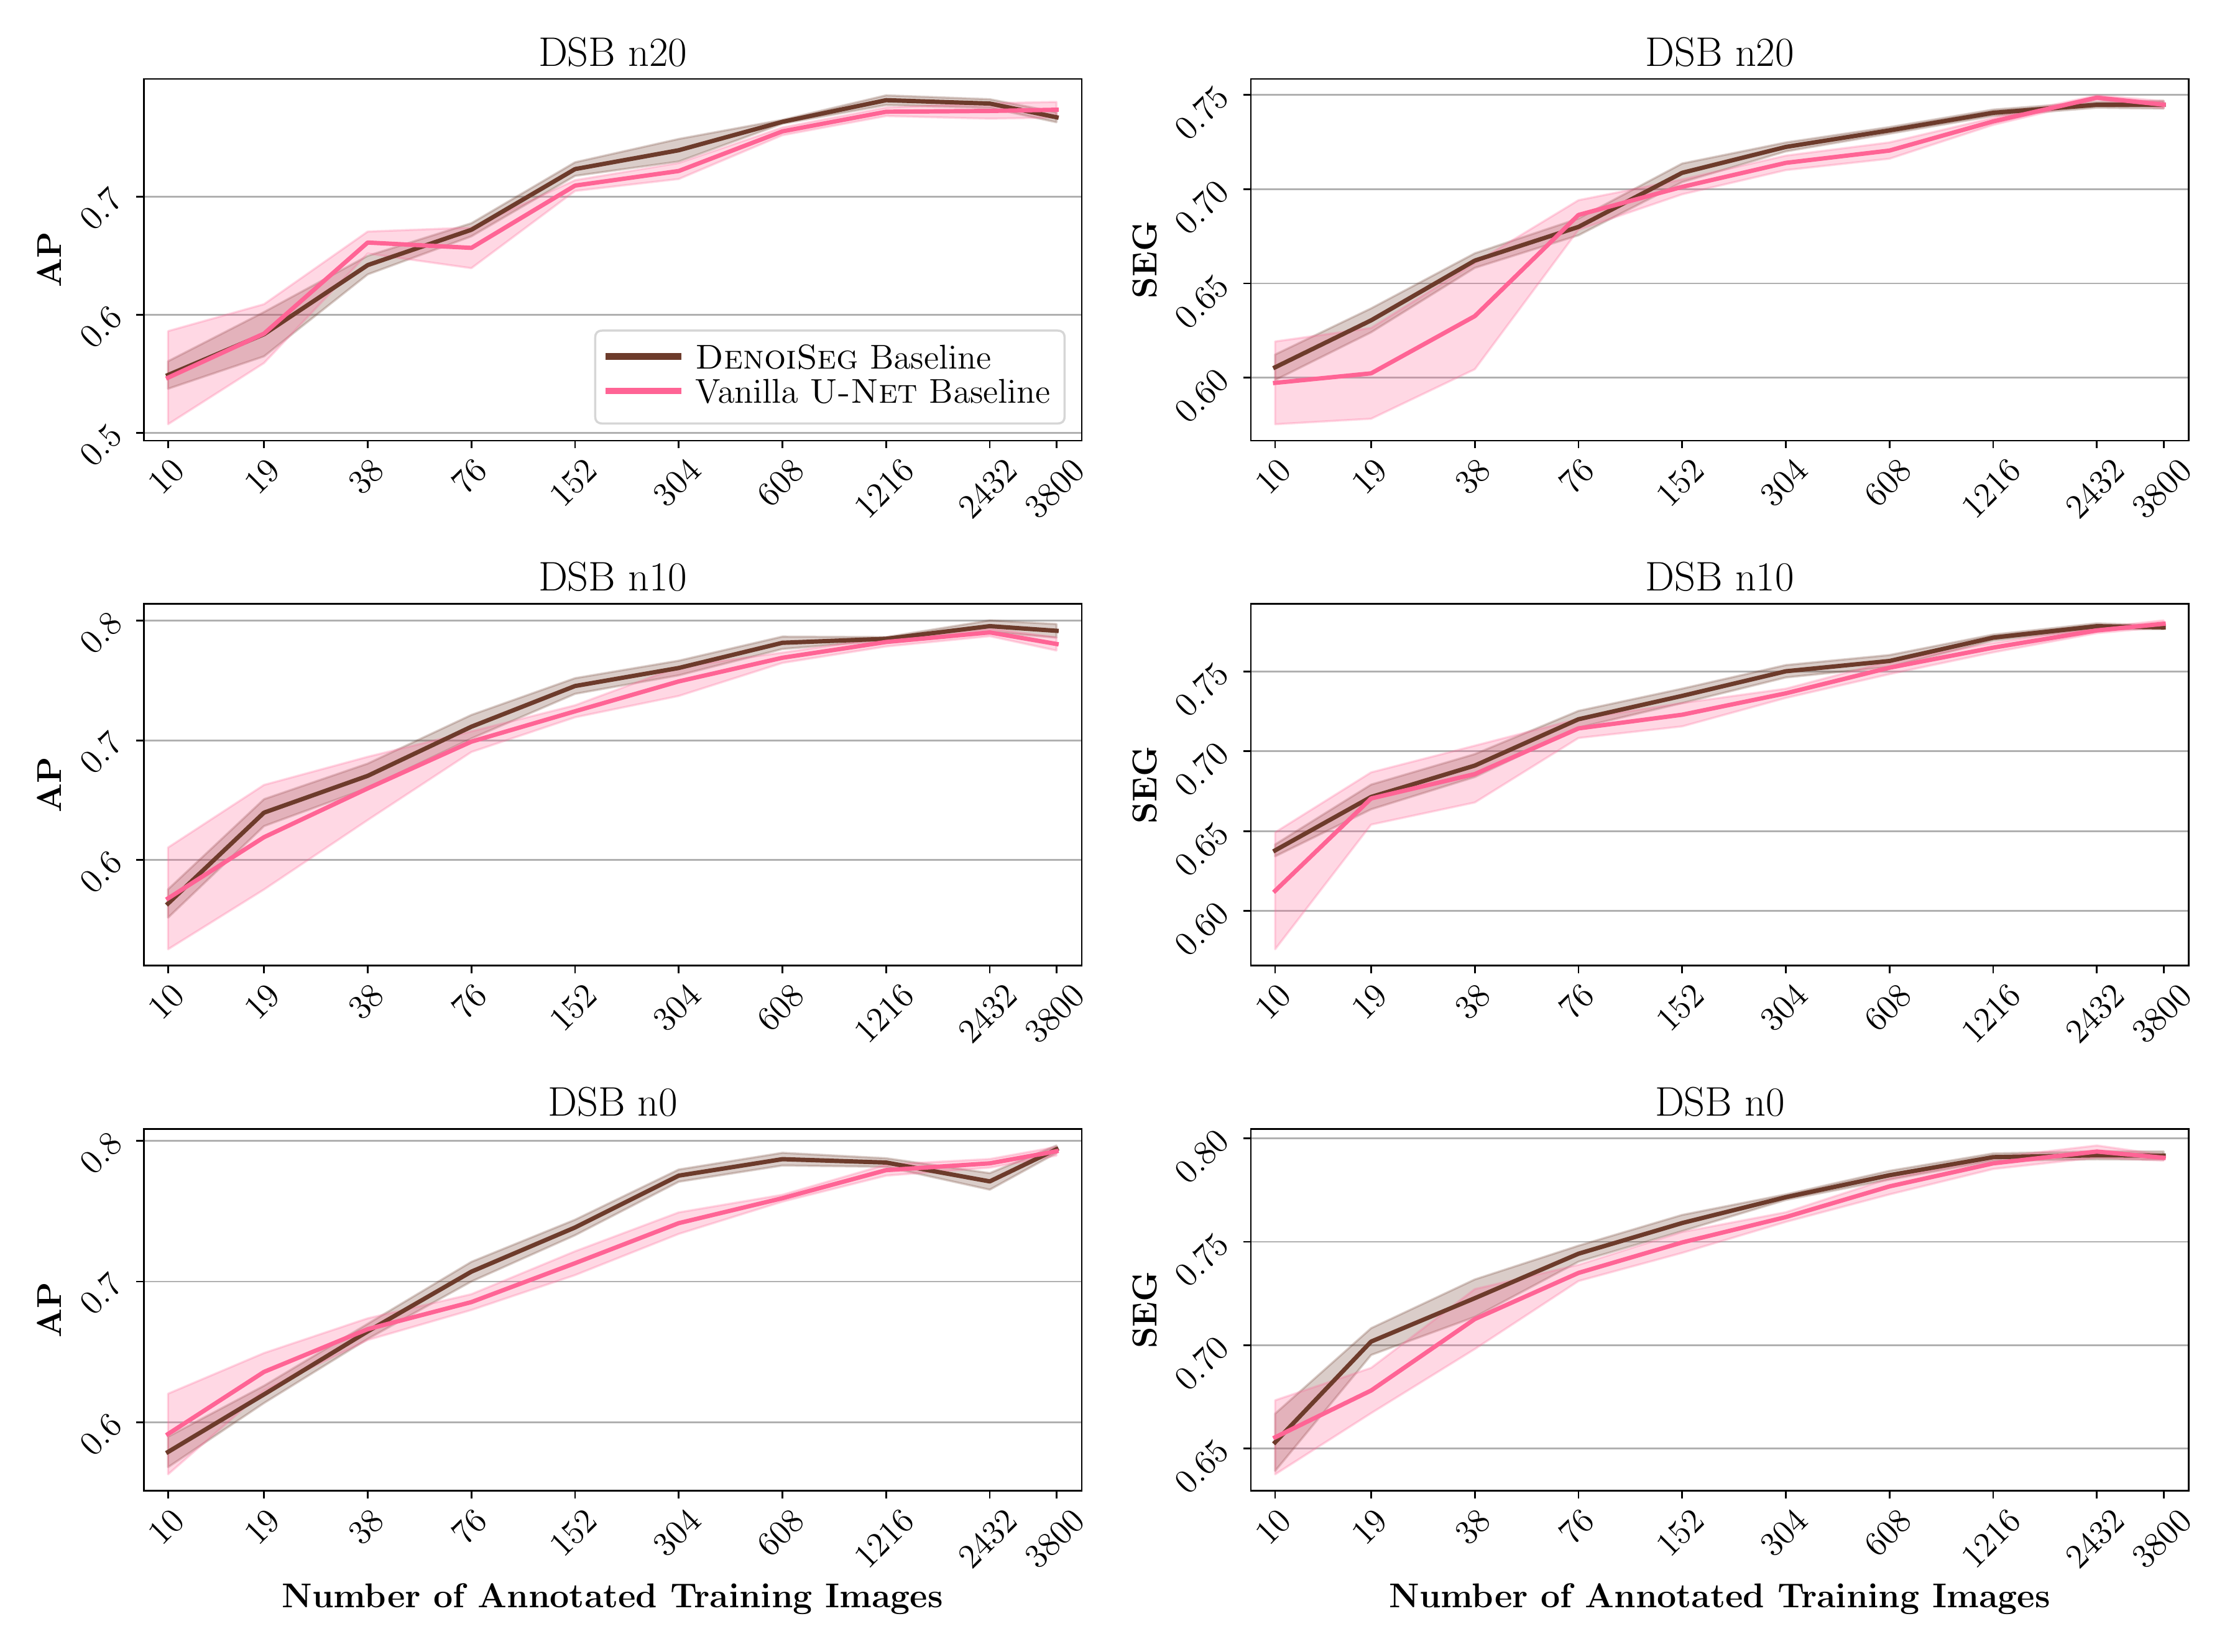}};
            \draw (-5.4, 4.2) node[inner sep=0] {(a)};
            \draw (0.35, 4.2) node[inner sep=0] {(b)};
        \end{tikzpicture}
    \end{minipage}
    
    \caption{Comparison of vanilla U-Net with our \DenoiSeg $\alpha=0$ baseline for DSB datasets.}
    \label{fig:vanillaBaseline}
\end{figure}
}

\begin{document}
\figFlyWing
\figMouseNuclei
\figDelta
\figVanillaBaseline
\end{document}
